# Supplementary material for: Crystalline membrane morphology beyond polyhedra
Source: arXiv:1903.00818 source file (2019-03-03)
Supplement: Supplementary file 1 [file membrane_static_SI.pdf]

# Supplementary Information

Hang Yuan

*Department of Materials Science and Engineering,*
*Northwestern University, Evanston, IL 60208*

Monica Olvera de la Cruz*

*Department of Materials Science and Engineering,*
*Northwestern University, Evanston, IL 60208*
*Department of Chemistry, Northwestern University, Evanston, IL 60208 and*
*Department of Physics and Astronomy,*
*Northwestern University, Evanston, IL 60208*

(Dated: March 3, 2019)

## Abstract

Supplementary information of the article: Crystalline membrane morphology beyond polyhedra. Contents are organized in following way:

**Magnetic energy expression:** This section provides derivations of the magnetic energy expression with the nearest neighbors approximation in the inextensible limit, i.e. equation (3) in the main text.

**Dimensionless parameters:** This section provides derivations of the Hamiltonian in dimensionless form and two dimensionless parameters: the Föppl-von Kármán parameter $\gamma$ and the magnetoelastic parameter $\Gamma$.

**Details of simulation setup:** This section provides details of the simulation setup and implementations of the volume constraint.

**Computation of curvatures:** This section explains how the curvatures of the membrane are computed from its configurational data.

**Membrane morphologies without the volume constraint:** This section shows the results of membrane morphologies without the volume constraint.

* m-olvera@northwestern.edu

## I. MAGNETIC ENERGY EXPRESSION

Comparing with the conventional elastic membranes, the energy of magnetoelastic membranes has an additional contribution from magnetic dipole-dipole interactions, which can be expressed as:

$$H_m = -\frac{\mu_0}{4\pi} \sum_{\mathbf{r}_i, \mathbf{r}_j \in \mathbf{V}, i \neq j} \frac{1}{|\mathbf{r}_{ij}|^3} \left[ 3 \left( \boldsymbol{\mu}_i \cdot \hat{\mathbf{r}}_{ij} \right) \left( \boldsymbol{\mu}_j \cdot \hat{\mathbf{r}}_{ij} \right) - \boldsymbol{\mu}_i \cdot \boldsymbol{\mu}_j \right] \tag{1}$$

where $\mu_0$ is the magnetic permeability in vaccum, $\boldsymbol{\mu}_i$ is the magnetic dipole moment at vertex $i$, $\mathbf{V}$ is the set of all vertices, $\mathbf{r}_i$ is the position vector of vertex $i$, $\mathbf{r}_{ij} = \mathbf{r}_j - \mathbf{r}_i$ and $\hat{\mathbf{r}}_{ij} = \mathbf{r}_{ij} / |\mathbf{r}_{ij}|$.

Since magnetic dipole-dipole interaction is long-range and anisotropic, we want to simplify the above expression. We assume the magnetic filed strength is strong enough that the induced magnetic dipole of each super-paramagnetic particles always aligns with the external magnetic field. For simplicity, we only consider the case where a magnetoelastic membrane is composed of the same type of super-paramagnetic particles. Then, the induced magnetic dipole moment of each super-paramagnetic particles is the same: $\boldsymbol{\mu}_i = \boldsymbol{\mu} = \mu \hat{\mathbf{m}}$, where $\hat{\mathbf{m}}$ is the direction of the external magnetic field.

The above magnetic dipole-dipole interactions term can be simplified by including only nearest neighbor interactions:

$$\begin{aligned} H_m &\approx -\frac{\mu_0}{4\pi} \sum_{\mathbf{r}_i, \mathbf{r}_j \in \mathbf{V}, i \neq j} \frac{1}{|\mathbf{r}_{ij}|^3} \left[ 3 \left( \boldsymbol{\mu} \cdot \hat{\mathbf{r}}_{ij} \right)^2 - \mu^2 \right] \\ &\approx -\frac{\mu_0}{4\pi} \sum_{\mathbf{r}_i \in \mathbf{V}} \sum_{\mathbf{r}_j \in \text{neighbors of i}} \frac{1}{|\mathbf{r}_{ij}|^3} \left[ 3 \left( \boldsymbol{\mu} \cdot \hat{\mathbf{r}}_{ij} \right)^2 - \mu^2 \right] \\ &= \frac{\mu_0 \mu^2}{4\pi} \sum_{\mathbf{r}_i \in \mathbf{V}} \sum_{\mathbf{r}_j \in \text{neighbors of i}} \frac{1}{|\mathbf{r}_{ij}|^3} \left[ 1 - 3 \left( \hat{\mathbf{m}} \cdot \hat{\mathbf{r}}_{ij} \right)^2 \right] \end{aligned} \tag{2}$$

Furthermore, we assume the membrane is inextensible, which means that the stretching constant is large enough thus all edge lengths are close to the equilibrium length $l_0$. With this assumption, all vertices are roughly equally distant and there are only two types of vertices: vertices with five neighbors(five-fold disclinations) and vertices with six neighbors. And the magnetic energy associated with each vertex type can be calculated accordingly:

1. Hexagonal vertex

   In this case, the vertices have six neighbors which locate on vertices of a regular

hexagon. Assuming the equilibrium length $l_0$ is small enough that locally six neighbors are in the same plane. By choosing z-axis as the normal direction of this regular hexagon(moving frame), locations of six neighbors can be written as $\hat{\mathbf{r}}_j = \left(\cos\frac{j\pi}{3}, \sin\frac{j\pi}{3}, 0\right), j = 0, \cdots, 5$ and the direction of the external magnetic field in this coordinate system can be expressed as $\hat{\mathbf{m}} = (r_t^i \cos\theta_t^i, r_t^i \sin\theta_t^i, m_n^i)$, where $r_t^i$ is the magnitude of in-plane component of $\hat{\mathbf{m}}$ at vertex $i$, $\theta_t^i$ is the corresponding polar angle in the plane and $m_n^i$ is the magnitude of out-plane component of $\hat{\mathbf{m}}$ at vertex $i$. Note that the components of $\hat{\mathbf{m}}$ in the chosen coordinate system depend on the location of vertex $i$. Then, the magnetic energy associated with each hexagonal vertex is

$$\begin{aligned}
\epsilon_{hex}^i &= \frac{\mu_0\mu^2}{4\pi} \sum_{j\in\text{neighbors of i}} \frac{1}{|\mathbf{r}_{ij}|^3} \left[1 - 3\left(\hat{\mathbf{m}} \cdot \hat{\mathbf{r}}_{ij}\right)^2\right] \\
&= \frac{\mu_0\mu^2}{4\pi} \sum_{j=0}^{5} \frac{1}{l_0^3} \left[1 - 3r_t^{i2} \left(\cos\theta_t^i \cos\frac{j\pi}{3} + \sin\theta_t^i \sin\frac{j\pi}{3}\right)^2\right] \\
&= \frac{\mu_0\mu^2}{4\pi} \sum_{j=0}^{5} \frac{1}{l_0^3} \left[1 - 3r_t^{i2} \cos^2\left(\theta_t^i - \frac{j\pi}{3}\right)\right] \\
&= \frac{\mu_0\mu^2}{4\pi} \frac{6}{l_0^3} \left[1 - \frac{3}{2} r_t^{i2}\right]
\end{aligned} \tag{3}$$

2. Pentagonal vertex

   By similarly choosing the coordinate system, the locations of neighbor vertices in the pentagonal case can be written as $\hat{\mathbf{r}}_j = \left(\cos\frac{2j\pi}{5}, \sin\frac{2j\pi}{5}, 0\right), j = 0, \cdots, 4$. The magnetic energy associated with each of the disclination vertices is:

$$\begin{aligned}
\epsilon_{pen}^i &= \frac{\mu_0\mu^2}{4\pi} \sum_{j\in\text{neighbors of i}} \frac{1}{|\mathbf{r}_{ij}|^3} \left[1 - 3\left(\hat{\mathbf{m}} \cdot \hat{\mathbf{r}}_{ij}\right)^2\right] \\
&= \frac{\mu_0\mu^2}{4\pi} \sum_{j=0}^{4} \frac{1}{l_0^3} \left[1 - 3r_t^{i2} \left(\cos\theta_t^i \cos\frac{2j\pi}{5} + \sin\theta_t^i \sin\frac{2j\pi}{5}\right)^2\right] \\
&= \frac{\mu_0\mu^2}{4\pi} \sum_{j=0}^{4} \frac{1}{l_0^3} \left[1 - 3r_t^{i2} \cos^2\left(\theta_t^i - \frac{2j\pi}{5}\right)\right] \\
&= \frac{\mu_0\mu^2}{4\pi} \frac{5}{l_0^3} \left[1 - \frac{3}{2} r_t^{i2}\right]
\end{aligned} \tag{4}$$

We consider a static external magnetic field pointing along the z-direction. Then, the direction of the external magnetic field is $\hat{\mathbf{m}} = (0, 0, 1)$ in the lab coordinate system. Denote the normal vector of i-th vertex as $\mathbf{n}_i$ and it can be expressed as $\hat{\mathbf{n}}_i = (n_x^i, n_y^i, n_z^i)$ in the lab

coordinate system. Thus, the in-plane component of $\hat{\mathbf{m}}$ at each vertex $i$ is:

$$\begin{aligned} {r_t^i}^2 &= [\hat{\mathbf{m}} - (\hat{\mathbf{m}} \cdot \hat{\mathbf{n}}_i)\hat{\mathbf{n}}_i]^2 = 1 - (\hat{\mathbf{m}} \cdot \hat{\mathbf{n}}_i)^2 \\ &= 1 - {n_z^i}^2 \end{aligned} \tag{5}$$

Plugging the above expression back into the energy expressions of the hexagonal vertex and the pentagonal vertex, we get

$$\epsilon_{hex}^i = 6\tilde{M}\left({n_z^i}^2 - \frac{1}{3}\right) \tag{6}$$

$$\epsilon_{pen}^i = 5\tilde{M}\left({n_z^i}^2 - \frac{1}{3}\right) \tag{7}$$

where $\tilde{M}$ gives the characteristic dipole-dipole interaction strength between a pair of nearest neighbors and is defined as:

$$\tilde{M} = \frac{1}{4}\frac{\mu_0}{4\pi}\frac{(3\mu)^2}{l_0^3}\frac{2}{3} \tag{8}$$

Then, putting all parts together gives the total magnetic energy of the membrane with the nearest neighbor approximation in the inextensible limit:

$$H_m \approx \left(\sum_{\mathbf{r}_i \in \mathbf{V}^{hex}} 6 + \sum_{\mathbf{r}_i \in \mathbf{V}^{pen}} 5\right)\tilde{M}\left({n_z^i}^2 - \frac{1}{3}\right) \tag{9}$$

We can bring the above discretization limit expression into the continuum limit by associating each vertex with its Voronoi cell area. The area of a regular hexagon with edge length $l_0$ is $\frac{3\sqrt{3}}{2}l_0^2$ and the corresponding Voronoi cell area of hexagonal vertex is $\frac{\sqrt{3}}{2}l_0^2$. Then, the magnetic energy density in the continuum limit is:

$$\epsilon_M = \frac{\epsilon_{hex}}{\frac{\sqrt{3}}{2}l_0^2} = \frac{1}{2}M\left(n_z^2 - \frac{1}{3}\right) \tag{10}$$

where the magnetic modulus $M$ is defined as

$$M = 2\sqrt{3}\frac{\mu_0}{4\pi l_0}\left(\frac{3\mu}{l_0^2}\right)^2\frac{2}{3} \tag{11}$$

Note that the above magnetic modulus has an addition factor of $2\sqrt{3}$ comparing with the result derived for square mesh[1]. The total magnetic energy in the continuum limit can be expressed as an integral of the magnetic energy density:

$$H_m \approx \int \frac{1}{2}M\left(n_z^2 - \frac{1}{3}\right)\mathrm{d}S \tag{12}$$

## II. DIMENSIONLESS PARAMETERS

With the derivations in the section I, the total magnetoelastic energy of the membrane in the discretization limit can be expressed as:

$$\begin{aligned} H_{em} &= \sum_{e\in\mathbf{E}} \frac{1}{2} k \left( |\mathbf{r}_1^e - \mathbf{r}_2^e| - l_0 \right)^2 + \sum_{e\in\mathbf{E}} \frac{1}{2} \tilde{\kappa} \left| \mathbf{n}_1^e - \mathbf{n}_2^e \right|^2 - \frac{\mu_0}{4\pi} \sum_{\mathbf{r}_i,\mathbf{r}_j\in\mathbf{V}, i\neq j} \frac{1}{|\mathbf{r}_{ij}|^3} \left[ 3 \left( \boldsymbol{\mu}_i \cdot \hat{\mathbf{r}}_{ij} \right) \left( \boldsymbol{\mu}_j \cdot \hat{\mathbf{r}}_{ij} \right) - \boldsymbol{\mu}_i \cdot \boldsymbol{\mu}_j \right] \\ &\approx \sum_{e\in\mathbf{E}} \frac{1}{2} k \left( |\mathbf{r}_1^e - \mathbf{r}_2^e| - l_0 \right)^2 + \sum_{e\in\mathbf{E}} \frac{1}{2} \tilde{\kappa} \left| \mathbf{n}_1^e - \mathbf{n}_2^e \right|^2 + \left( \sum_{\mathbf{r}_i\in V^{hex}} 6 + \sum_{\mathbf{r}_i\in\mathbf{V}^{pen}} 5 \right) \tilde{M} \left( {n_z^i}^2 - \frac{1}{3} \right) \end{aligned} \tag{13}$$

where $k$ is the microscopic stretching constant, $\tilde{\kappa}$ is the microscopic bending constant and $\tilde{M}$ is the microscopic characteristic dipole-dipole interaction strength. By choosing the unit energy as $\tilde{\kappa}$ and the unit length as $R$ (radius of the initial spherical shell), the above expression becomes dimensionless:

$$\begin{aligned} \tilde{H}_{em} &= \sum_{e\in\mathbf{E}} \frac{1}{2} \frac{kR^2}{\tilde{\kappa}} \left( \left| \tilde{\mathbf{r}_1^e} - \tilde{\mathbf{r}_2^e} \right| - \tilde{l_0} \right)^2 + \sum_{e\in\mathbf{E}} \frac{1}{2} \left| \mathbf{n}_1^e - \mathbf{n}_2^e \right|^2 + \left( \sum_{\mathbf{r}_i\in V^{hex}} 6 + \sum_{\mathbf{r}_i\in\mathbf{V}^{pen}} 5 \right) \frac{\tilde{M}}{\tilde{\kappa}} \left( {n_z^i}^2 - \frac{1}{3} \right) \\ &= \sum_{e\in\mathbf{E}} \frac{1}{2} \tilde{\gamma} \left( \left| \tilde{\mathbf{r}_1^e} - \tilde{\mathbf{r}_2^e} \right| - \tilde{l_0} \right)^2 + \sum_{e\in\mathbf{E}} \frac{1}{2} \left| \mathbf{n}_1^e - \mathbf{n}_2^e \right|^2 + \left( \sum_{\mathbf{r}_i\in V^{hex}} 6 + \sum_{\mathbf{r}_i\in\mathbf{V}^{pen}} 5 \right) \tilde{\Gamma} \left( {n_z^i}^2 - \frac{1}{3} \right) \end{aligned} \tag{14}$$

Note that the above Hamiltonian has two dimensionless parameters $\tilde{\gamma} = \frac{kR^2}{\tilde{\kappa}}$ and $\tilde{\Gamma} = \frac{\tilde{M}}{\tilde{\kappa}}$, which give characteristic interaction strengths in the microscopic scale. We can also bring the system into the continuum limit, which gives two more familiar dimensionless parameters of the system:

$$\gamma = \frac{YR^2}{\kappa}, \Gamma = \frac{MR^2}{\kappa} \tag{15}$$

where $\gamma$ is the Föppl-von Kármán parameter, which gives characteristic relative strength between stretching interaction and bending interaction. $\Gamma$ is the magnetoelastic parameter, which gives characteristic relative strength between magnetic dipole-dipole interaction and bending interaction. Correspondences between parameters in the discretization limit and the continuum limit[2, 3] are listed below:

$$Y = \frac{2k}{\sqrt{3}}, \kappa = \frac{\tilde{\kappa}}{\sqrt{3}}, M = \frac{8\sqrt{3}}{l_0^2} \tilde{M} \tag{16}$$

## III. DETAILS OF SIMULATION SETUP

The simulations are performed in LAMMPS[4]. All interactions in the Hamiltonian of the system can be mapped to commonly available interactions in LAMMPS. More specifically, stretching interactions are modeled as harmonic bond interactions, bending interactions are modeled as harmonic dihedral interactions, and magnetic dipole-dipole interactions are modeled as electric dipole-dipole interactions (both are equivalent in reduced units). Shifted Lennard-Jones interactions are included to account for finite size effect of the super-paramagnetic particles and to increase the stability of the collapsed state simulation. The cutoff of the Lennard-Jones interactions is set as 0.6 of equilibrium length $l_0$.

Each vertex is represented as a point dipole in the simulations. The computation of the long range magnetic dipole-dipole interactions is performed without a cutoff. Because of properties of super-paramagnetic particles, directions of each dipole are always aligned with the external magnetic field. Besides, only translational degrees of freedom are updated in each timestep. Rotational degrees of freedom of each vertex are ignored because super-paramagnetic particles don't have permanent magnetization which decouples magnetics and elasticity.

Initial mesh of the membrane is constructed with the scheme proposed by Caspar and Klug[5]. Different mesh choices (different h,k numbers) are tested to ensure that observed phenomena are not mesh dependent. All simulations mentioned in this paper are performed with mesh $(6, 6)$, which has 1082 vertices, 3240 edges and 2160 faces. The simulations are performed with typical annealing process to get minimum energy configuration of the magnetoelastic membranes. The annealing process is repeated for five times to ensure the final membrane configuration is not trapped in local minima.

The volume constraint is added when the membrane is not penetrable, which is implemented as a fix package of LAMMPS. An additional potential energy from the volume constraint is modeled as following:

$$H_v = \Lambda \left( \sum_k \Omega_k - V_{ref} \right)^2 \tag{17}$$

where $\Omega_k$ is the signed volume of the tetrahedron extended by k-th triangle on the membrane, $V_{ref}$ is the reference volume of the membrane and $\Lambda$ is the Lagrange multiplier. Then, taking derivatives of the above potential with respect to each vertex gives the constraint forces from

the volume constraint. For example, consider a triangle consists of three vertices: $\mathbf{r}_1, \mathbf{r}_2, \mathbf{r}_3$. The signed volume of the tetrahedron extended by this triangle is:

$$\Omega_k = \frac{1}{6}\mathbf{r}_1 \cdot \mathbf{r}_2 \times \mathbf{r}_3 \tag{18}$$

Then, taking derivatives of $\Omega_k$ with respect to $\mathbf{r}_1$ is

$$\nabla\Omega_k|_{\mathbf{r}_1} = \frac{1}{6}(-y_3z_2 + y_2z_3, x_3z_2 - x_2z_3, -x_3y_2 + x_2y_3) \tag{19}$$

Other cases are cyclic permutations of the above result. Note that the interaction from the volume constraint is not pair-like interaction and total constraint force of vertex $i$ is:

$$f^{(i)}_{constraint} = 2\Lambda \sum_{k \in \text{neighbors of i}} \nabla\Omega_k|_{\mathbf{r}_i} \tag{20}$$

## IV. COMPUTATION OF CURVATURES

Computation of curvatures generally requires a surface is differentiable. However, in the discretization limit, the surface is composed of flat triangles and is a piece-wise constant surface, which has only $C^0$ continuity. Then, computation of curvatures on the triangulated surface needs additional considerations.

The method used in this paper to compute the curvatures of the magnetoelastic membranes follows the work of Meyer et al[6], which is introduced in the context of computer graphics. By associating each vertex with its corresponding Voronoi cell, the mean curvature vector $\mathbf{K}$ and the gaussian curvature $\kappa_G$ are calculated by following formulae:

$$\mathbf{K}(\mathbf{r}_i) = \frac{1}{2A(\mathbf{r}_i)} \sum_{j \in \text{neighbors of i}} (\cot\alpha_{ij} + \cot\beta_{ij})(\mathbf{r}_i - \mathbf{r}_j) \tag{21}$$

$$\kappa_G(\mathbf{r}_i) = \left(2\pi - \sum_{j \in \text{external angles}} \theta_j\right) / A(\mathbf{r}_i) \tag{22}$$

where $\alpha_{ij}$ and $\beta_{ij}$ are two angles opposite to the edge defined by vertices $\mathbf{r}_i$ and $\mathbf{r}_j$. $A(\mathbf{r}_i)$ is the area of Voronoi cell of vertex $i$:

$$A(\mathbf{r}_i) = \frac{1}{8} \sum_{j \in \text{neighbors of i}} (\cot\alpha_{ij} + \cot\beta_{ij}) |\mathbf{r}_i - \mathbf{r}_j|^2 \tag{23}$$

and $\theta_j$ are the external angles of the Voronoi cell around vertex $i$. Note that when triangles are obtuse, $A(\mathbf{r}_i)$ needs to be modified[6] to make sure that Voronoi cells are non-overlapping,

which in turn makes sure that the sum of Gaussian curvature fulfills the Gauss-Bonnet theorem. By comparing the direction of mean curvature vector $\mathbf{K}$ with the exterior normal direction of the membrane, a sign can be associated with the mean curvature value to distinguish convex and concave regions of the membrane.

## V. MEMBRANE MORPHOLOGIES WITHOUT THE VOLUME CONSTRAINT

We also explore the cases without the volume constraint, which correspond to the situation that materials inside the membrane can freely penetrate the membrane. Possible morphologies of the membranes without the volume constraint are shown in Fig. 1.

Comparing with the results of the cases with the volume constraint, the volume constraint

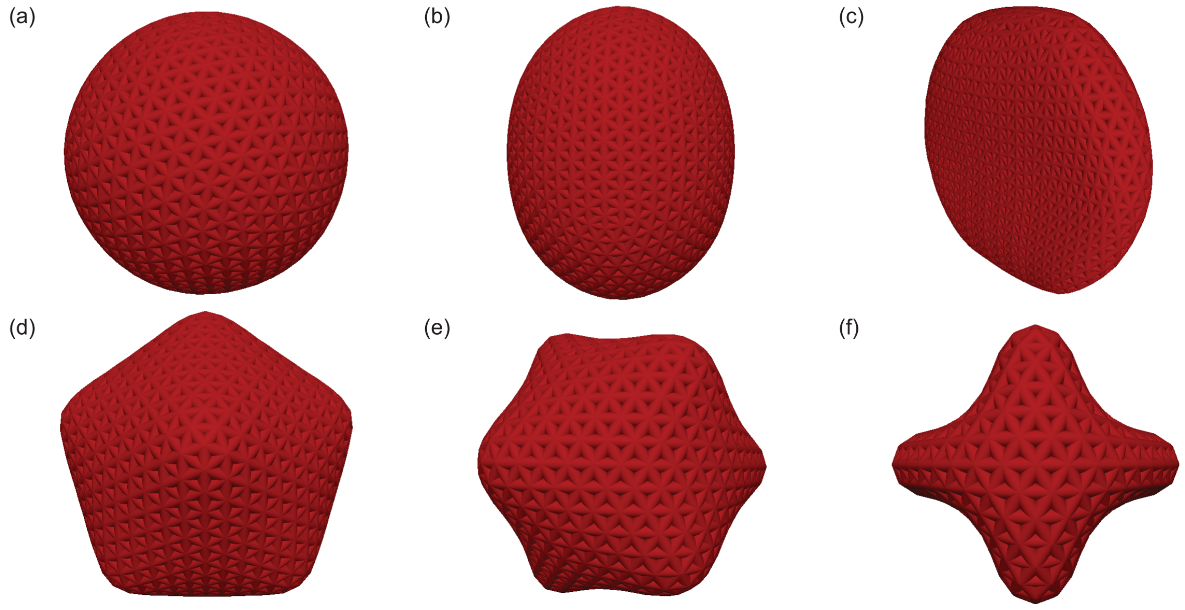


FIG. 1. A collection of representative minimum energy morphologies of the closed magnetoelastic membrane without the volume constraint. Different parameters pairs $(\gamma, \Gamma)$, Föppl-von Kármán parameter $\gamma$ and magnetoelastic parameter $\Gamma$, are explored. $\gamma$ increases from top to bottom and $\Gamma$ increases from left to right. (a) spherical shape (100,0); (b) ellipsoidal shape (100,20); (c) pancake shape (100,40); (d) icosahedral shape (1000,0); (e) star shape with six ridges (1000,80); (f) star shape with four ridges (1000,150). Note that (a) and (b) are shown from y-direction, (c) is shown from angled view and second row is shown from z-direction to give better illustration of morphologies.

shifts the transition points between different morphologies, which is expected and controlled by the parameters $V_{ref}$ and $\Lambda$. The morphologies without the volume constraint generally do not differ significantly from the cases with the volume constraint, except the cases in the high field strength limit.

For example, as shown in Fig. 1c, the membrane morphology becomes "pancake" shape when the membrane is relatively soft ($\gamma < \gamma^*$) in the high field strength limit. The "pancake" shape brings magnetic dipoles even closer than cylindrical shape(corresponding morphology with the volume constraint) since there is no additional volume constraint to prevent the membrane from shrinking.

When the membrane is relatively stiff ($\gamma > \gamma^*$) in the high field strength limit, many crumpled states or collapsed states are observed as shown in Fig. 2. These morphologies are difficult to describe and generally differ a lot from each other. The magnetoelastic membranes in those cases are highly nonlinear and both magnetic and elastic energy are significant. Small fluctuations of the membrane disclinations can change the membrane morphology significantly in those cases and lead to different crumpled states or collapsed states. Without the volume constraint, the membranes resist magnetic dipole-dipole interactions

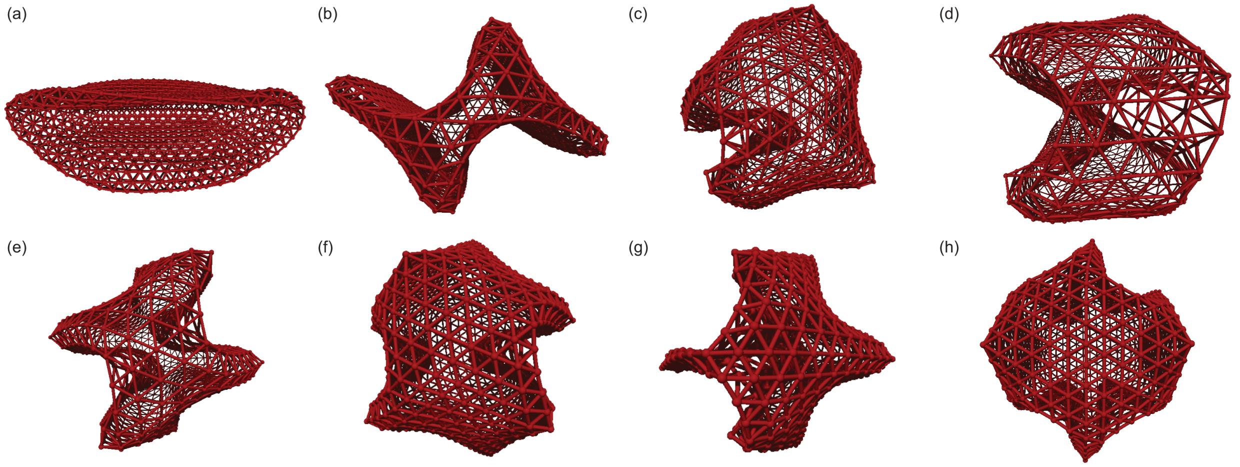


FIG. 2. Examples of crumpled states and collapsed states. These morphologies are observed in the cases without the volume constraint in the high magnetic field strength limit. Morphologies in these cases are presented by triangulation mesh to give better illustration. Their corresponding parameters pairs $(\gamma, \Gamma)$ are: (a) (1000,200); (b) (2000,600); (c) (4000,200); (d) (5000, 300); (e) (6000,500); (f) (8000,200) (g) (10000,500) (h) (50000,400). Note that (a) is shown in angled view while others are shown in z-direction.

by elasticity(although Lennard-Jones interactions also help stabilizing the membrane when the membrane is collapsed). After reaching certain magnetic field strength, the membranes cannot hold a definite shape anymore and are free to crumple or collapse since there is no volume constraint to restrict these crumpling or collapsing processes. This creates a family of complicated morphologies with a few selected examples as shown in Fig. 2. It is interesting to notice that these morphologies in Fig. 2 ($\gamma > \gamma^*$ in high magnetic field strength limit), still roughly maintain two-fold symmetry for some states (Fig. 2b, d, e, f and h). In contrast, the membranes with the volume constraint in high magnetic field strength limit collapse into morphologies with three-fold and two-fold rotational symmetry only and never take crumpled shapes shown in Fig. 2. If the membrane is not penetrable, a volume constraint is needed to consider the internal pressure of the membrane as discussed in the main text. With the existence of the volume constraint, all those crumpled states and collapsed states(Fig. 2) found in penetrable membranes become much more well-defined morphologies with three-fold or two-fold symmetry as discussed in the main text. When the strength of the external magnetic field becomes extremely strong, the membrane with the volume constraint collapses into the morphology with only one-fold rotational symmetry.

---


[1] Pablo Vázquez-Montejo and Mónica Olvera de la Cruz. Flexible paramagnetic membranes in fast precessing fields. *Phys. Rev. E*, 98:032603, Sep 2018.

[2] H. S. Seung and David R. Nelson. Defects in flexible membranes with crystalline order. *Phys. Rev. A*, 38:1005–1018, Jul 1988.

[3] D. R. Nelson, T. Piran, and S. Weinberg. *Statistical Mechanics of Membranes and Surfaces*. World Scientific Pub., 2004.

[4] Steve Plimpton. Fast parallel algorithms for short-range molecular dynamics. *Journal of Computational Physics*, 117(1):1–19, March 1995.

[5] D. L. D. Caspar and A. Klug. Physical principles in the construction of regular viruses. *Cold Spring Harbor Symposia on Quantitative Biology*, 27:1–24, 1962.

[6] Mark Meyer, Mathieu Desbrun, Peter Schrder, and Alan H. Barr. Discrete differential-geometry operators for triangulated 2-manifolds. In Hans-Christian Hege and Konrad Polthier, editors, *Visualization and Mathematics III*, pages 35–57, Berlin, Heidelberg, 2003. Springer Berlin Hei-

delberg.
